# Supplementary material for: Action Anticipation with RBF Kernelized Feature Mapping RNN
Source: arXiv:1911.07806 source file (2021-07-11)
Supplement: Supplementary file 1 [file 6supplementary.tex]

\section*{APPENDIX A: Inference}

\begin{figure}[h]
      \centering
      \includegraphics[width=0.3\textwidth]{images/inference.PNG}
      \caption{Inference of Time Series-based LSTM Processing Models}\label{fig:itslpm}
\end{figure}

Let Fig.~\ref{fig:itslpm} be an example of the results acquired from the LSTM model. In this particular case, the dataset contains 6 different classes and the Neural Network processes 4 frames of feature at a time. We propose two different inference schemes implemented with different pooling methods:
\begin{itemize}
\item[] \textbf{Average Pooling:} The label of the frame $l$ (a scalar that represents the class) is decided by taking the average probability of each label over all 4 time steps and finding the index in  $\boldsymbol{\hat{l}_t}$ with maximum probability, i.e.\par 
\begin{center}
$l=argmax(\boldsymbol{\hat{l}_t})$, where $\boldsymbol{\hat{l}_t}=p^k = \frac{1}{T}\displaystyle\sum_{i=1}^T{p^k_{t_i}}$
\end{center}

\item[] \textbf{Max Pooling:} The label of the frame $l$ is decided by taking the maximum probability of each label over all 4 time steps and finding the index in  $\boldsymbol{\hat{l}_t}$ with maximum probability, i.e.\par 
\begin{center}
$l=argmax(\boldsymbol{\hat{l}_t})$, where $\boldsymbol{\hat{l}_t}=p^k = max({p^k_{t_i}})$
\end{center}
\end{itemize}
It is not hard to imagine that one usually acquires higher accuracy with average pooling, as it takes all the classification results of all $T$ time steps into consideration. However, information can be lost while smoothing the data, which makes outliers harder to be detected. Since this is not optimal for model training, max pooling is also used in accuracy evaluation for a more representative measurement of the model's performance. The accuracy acquired from average pooling, max pooling and without pooling are all reported.

\section*{Appendix B: Correlation Analysis}

As mentioned previously, for the feature matching RNN to work, there must exists some kind of correlation between the values of features created by \textit{Inception V3}. To confirm our theory, correlation matrices are calculated between segments of features, with length of segments ranging from $2^3$ to $2^{10}$ with increment of $8$. Note that the "segments of features" investigated here are equivalent to the feature step size in Fig.~\ref{sec:featurestepsize}. Some of the correlation matrices are visualised on hot-map and shown in Fig.~\ref{fig:vcmdfss}.
\begin{figure}[h]
      \centering
    \begin{subfigure}[b]{0.23\textwidth}
        \centering
        \includegraphics[width = \textwidth]{images/32.png}
        \caption{Feature Step Size $D=32$}\label{fig:32}        
    \end{subfigure}
    \begin{subfigure}[b]{0.23\textwidth}
        \centering
        \includegraphics[width = \textwidth]{images/64.png}
        \caption{Feature Step Size $D=64$}\label{fig:64}
    \end{subfigure} \\
    \begin{subfigure}[b]{0.23\textwidth}
        \centering
        \includegraphics[width = \textwidth]{images/128.png}
        \caption{Feature Step Size $D=128$}\label{fig:128}
    \end{subfigure}  
    \begin{subfigure}[b]{0.23\textwidth}
        \centering
        \includegraphics[width = \textwidth]{images/256.png}
        \caption{Feature Step Size $D=256$}\label{fig:256}
    \end{subfigure}  
    \begin{subfigure}[b]{0.23\textwidth}
        \centering
        \includegraphics[width = \textwidth]{images/416.png}
        \caption{Feature Step Size $D=416$}\label{fig:416}     
    \end{subfigure}
    \begin{subfigure}[b]{0.23\textwidth}
        \centering
        \includegraphics[width = \textwidth]{images/424.png}
        \caption{Feature Step Size $D=424$}\label{fig:424}
    \end{subfigure} 
    \caption{Visualisation of Correlation Matrix for Different Feature Step Size} \label{fig:vcmdfss}
\end{figure}
Note that we set all diagonal values of the correlation matrices from to 0 to make the results more distinctive on the hot-map plot (originally all $1$). An overlapping of the brighter region, which indicates higher correlations, can be observed especially in Fig.~\ref{fig:128} and Fig.~\ref{fig:256}, which proves the consistency of the levels of correlation between segments of features at different part of the vector. We can also see that the larger the feature step size is, the dimmer the hot-mat plot, which indicates a negatively-proportional relationship between correlation level and feature step size. If we plot the average value of the entire correlation matrix against the feature step size, we will find that the average value of correlation matrix decreases as feature step size increase, as shown in \Fref{fig:avocm}. 
\begin{figure}[h]   
        \centering
        \includegraphics[width = 0.35\textwidth]{images/correlation_average.png}
        \caption{Average Value of Correlation Matrix vs. Feature Step Size}\label{fig:avocm}      
\end{figure}
To further investigate this relationship, we can use the results in previous section on the relationship between feature step size and prediction accuracy. Take feature step size $416$ and $424$ as an example, as shown in the below images. Although \Fref{fig:424} is acquired with larger feature step size, its hot-map plot shows a much more distinctive correlation than in \Fref{fig:416}. This is also reflected on the prediction accuracy of the two step sizes, with $25.7\%$ when $D=416$ and $78.9\%$ when $D=424$.

\section*{Appendix C:}

Plots of RNN total loss at different feature step size in the training process can be found in Fig.~\ref{fig:tl}. Again, significant oscillation can be observed, especially when training using smaller feature step size. A possible explanation for this is that the significance of each feature segment to the task of future feature generation are different, and that weight sharing among features is not a perfect fit for the data at all times. From Fig.~\ref{fig:tl} we can clearly observe that when the feature step size becomes larger, the optimisation of the model in each step is more consistent, which results in the decrease of oscillation magnitude.

\begin{figure}[h]
      \centering
      \includegraphics[width=0.35\textwidth]{images/LSTM_tl.png}
      \caption{Loss during training at different feature step size using \textit{JHMDB-21} dataset}\label{fig:tl} 
\end{figure} 

The loss of feature matching RNN during training process using three different feature step size (16, 480 and 976) can be found in Fig.~\ref{fig:tl}. Here, significant oscillation can be observed especially with smaller feature step size. A possible explanation for this is that some of the feature segments are more relevant for the task of future feature generation than others, which is demonstrated as significant inconsistency in training loss due to the different levels of training stabilisation difficulty; this assumption can also explain why models with smaller feature step size are more preferable than large ones: when training on small group of features, the RNN is able to focus on the key clusters of features that contains information about action and optimises the corresponding network parameters easily; as a result, even if the training cost of some steps are high,  since the effect of their corresponding feature segments is minimal to the feature prediction and generation task, high accuracy is guaranteed as long as the prediction to action-relevant features have lower costs. When feature step size is large, the model tries to regularise a large set of features with mixed information at one time step, which results in longer training time and lower prediction accuracy. We deliberately chose $D=480$ and $D=976$ in Fig.~\ref{fig:tl} to showcase such an example: it is clearly shown in the plot that the former has higher average loss than the latter, however the accuracy when $D=480$ is roughly $50\%$ higher than when $D=976$.
\par

\section*{Appendix D}
The motivation of this can be demonstrated by the binary classification problem depicted in Fig.~\ref{fig:ksls}. In this plot, we can see that linear SVM can only separate data with hyperplane (in this case, a straight line); kernel SVMs, on the other hand, has the ability of separating clusters with more complex shapes by combining Gaussian surfaces to form the boundaries, and therefore has significantly lower classification error than linear SVM.

\begin{figure}[h]
      \centering
      \includegraphics[width=0.25\textwidth]{images/motivation.png}
      \caption{Kernel SVM vs. Linear SVM}\label{fig:ksls}       
\end{figure}
